# Supplementary material for: Multiplex Behavioral Relation Learning for Recommendation via Memory Augmented Transformer Network
Source: arXiv:2110.04002 source file (2021-10-08)
Supplement: Supplementary file 1 [file appendix.tex]

\section{Appendix}
\label{sec:appendix}
